# Supplementary material for: Pixels and Predictions: Potential of GPT-4V in Meteorological Imagery Analysis and Forecast Communication
Source: arXiv:2404.15166 source file (2024-09-07)
Supplement: Supplementary file 1 [file GPT_supplementary.pdf]

**Prompt:**
I am going to pass pairs of weather-forecast maps to you, one from NAM and one from GFS weather models each time (see top right corner for which model), over the continental US. Silently assess each pair as I enter them, and eventually I will ask you to summarise the regions of uncertainty between the two predicted future states. I will then ask which variables, pressure levels, etc would help you improve your analysis on atmospheric uncertainty. Please focus on things like surface-pressure lows/highs, likely precipitation areas and type of precipitation, other dangerous weather conditions, and so on. You are a weather expert speaking to fellow experts.

---

[This text not part of prompt. The images are 60-h forecasts of

- 300 hPa geopotential height and wind
- 500 hPa and 850 hPa dry-bulb temperature, geopotential height, wind
- Mean sea-level pressure, 2-m equivalent potential temperature, 10-m wind
- Simulated composite reflectivity

shown after this box. NAM is left column, GFS is right.]

---

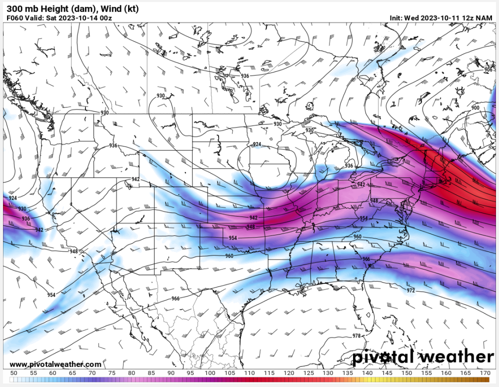


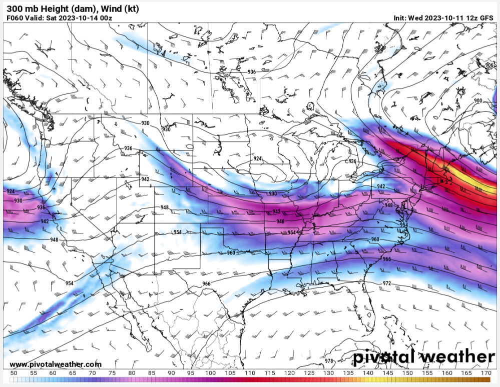


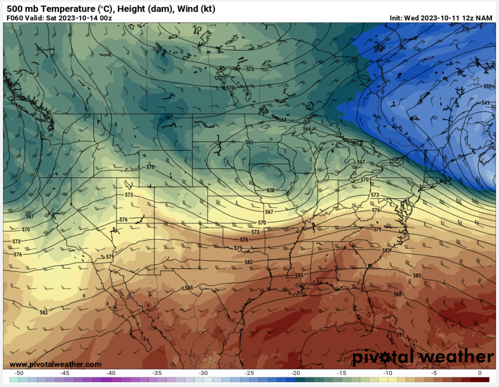


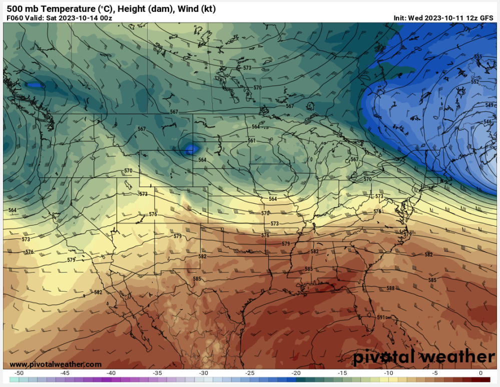

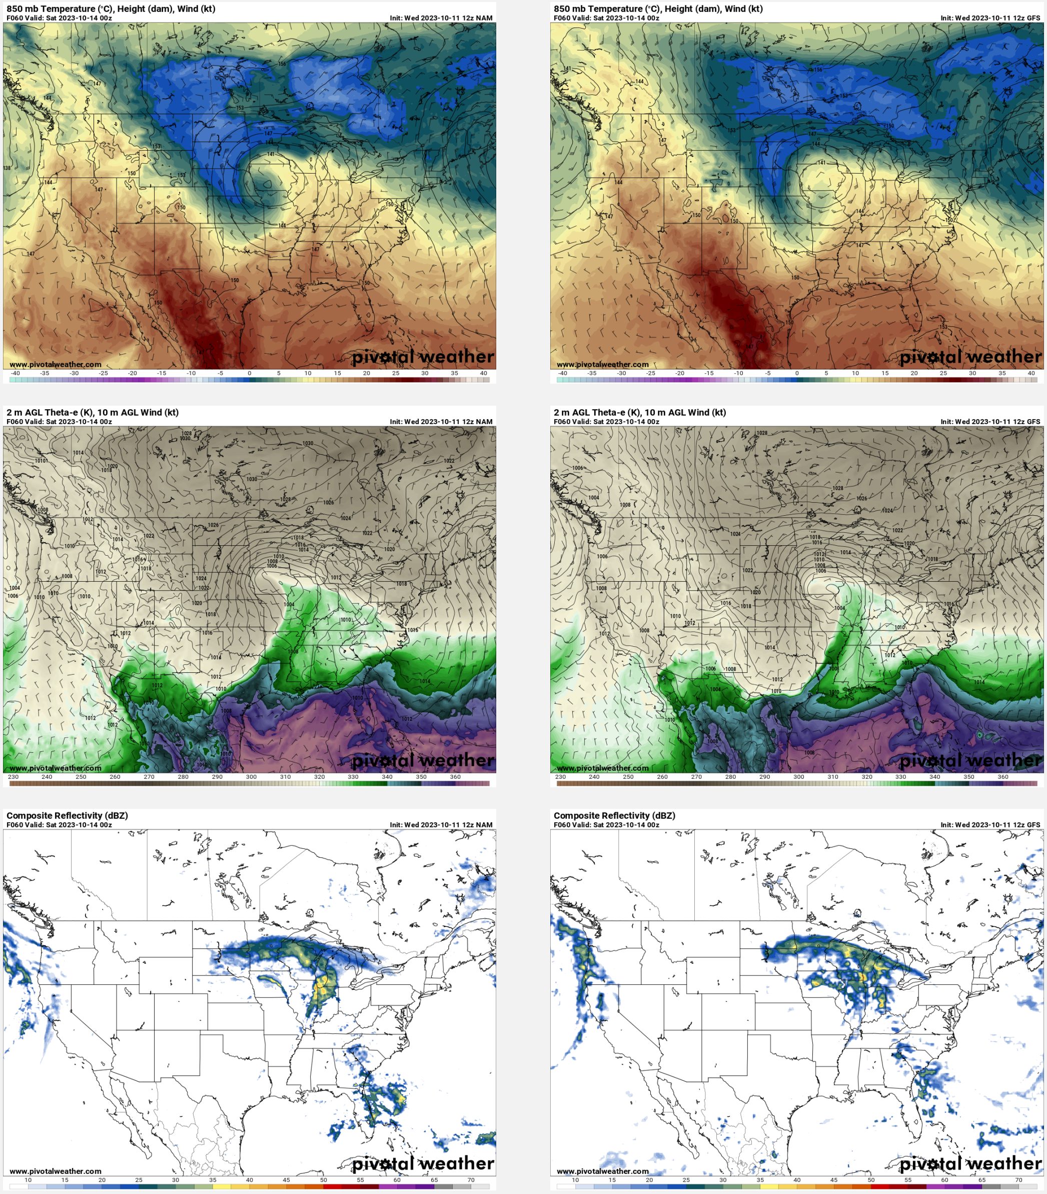


Now, please compare these forecasts and how it gives the forecaster a sense of inherent uncertainty in the forecast for 60 hours' time after synthesising all variables, levels, etc. Also tell me which further maps I can give you to improve your evaluation.

**GPT-4V:**

[*ChatGPT responded to the image prompts with a concise acknowledgment. It was then prompted after the last pair of images to continue.*]

Certainly. Let's evaluate the inherent uncertainty between the NAM and GFS models from the sets of maps provided:

- **Surface-level: Pressure and Precipitation**. There are some differences in the placement and intensity of the surface pressure lows and highs between the two models. The NAM seems to show more pronounced pressure troughs and ridges. In terms of precipitation, while the general patterns align (e.g., potential rain/storms in the Eastern US), the intensity and exact placement vary slightly.
- **500mb Level: Temperature, Height, and Wind**. Both models showed troughs and ridges, but their positions were slightly offset. This can lead to differences in the forecasted weather, as the position of these features can greatly influence surface weather conditions. The temperatures at this level also had minor differences, which might affect instability and cloud formation predictions.

- **850mb Level: Temperature, Height, and Wind**. There are differences in the predicted temperature gradients, especially in the central US. The wind patterns are somewhat similar, but there are discrepancies in the intensity and flow direction. This level is crucial for understanding moisture transport and frontal boundaries, so discrepancies here could lead to differences in precipitation forecasts.
- **300mb Level: Jet Stream (Wind) and Heights**. Differences can be noticed in the jet stream's position and intensity, with the NAM indicating a more pronounced jet streak over the northeastern US. The jet stream plays a significant role in steering weather systems, so differences here can impact the forecasted track of systems.
- **Composite Reflectivity: Precipitation**. The patterns of predicted precipitation broadly align in the larger sense, but there are evident differences in intensity and exact placement. For example, the intensity of the system over the northeastern US differs between the models.

In terms of improving the evaluation, having access to the following additional maps would be beneficial:

1. **Upper Air Soundings**: These provide a vertical profile of the atmosphere and can help in understanding stability, potential for convection, and cloud formation.
2. **Surface Dew Points**: This will give insights into moisture availability, which is crucial for convection and precipitation forecasts.
3. **Sea Level Pressure and Frontal Boundaries**: This can give a clearer picture of the position and movement of high and low-pressure systems, as well as cold, warm, occluded, and stationary fronts.
4. **Vorticity at 500mb**: This helps in identifying areas of potential rotation or spin in the atmosphere, often associated with storm development.
5. **Specific Humidity or Relative Humidity Maps**: These would provide a sense of the moisture distribution in the atmosphere.

---

**Prompt:**
1. Did you synthesise the equivalent potential temperature (theta-e) from the first plot?
2. Can you be more specific in terms of differences and specific weather phenomena (such as fronts and low-pressure centres)? There is little utility in pointing out that differences exist as they always will do. It is the magnitude and character of differences compared to "typical" that is more interesting. Please use numerical values where relevant, such as differences in local minima in surface pressure.
3. Attached is a pair of images so you can update your 3-D internalisation of the atmosphere [Not part of prompt: these are 700-hPa forecast charts of relative humidity.]
4. I would like you to infer things like cold/warm fronts from the data I've already given, unless you are missing essential data to do so.

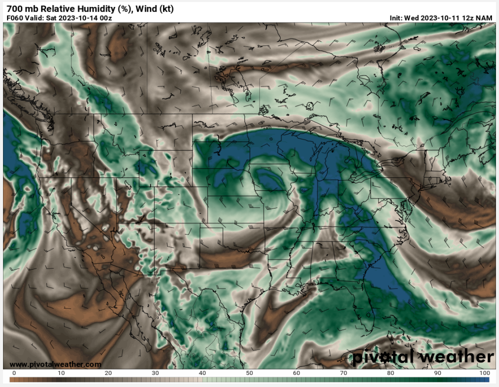


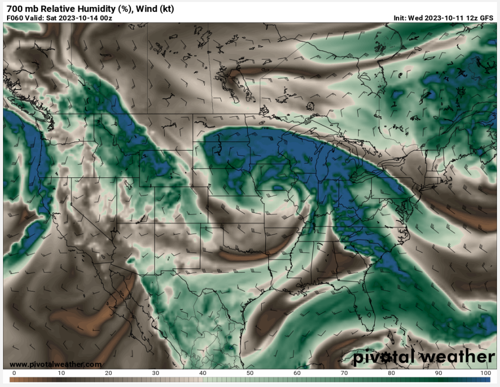


Please regenerate your analysis of uncertainty with this new information and updated instructions. Don't be afraid to say "I don't know" if you cannot identify required information in the maps I gave, as I can pass more images in if required.

**GPT-4V:**
Equivalent Potential Temperature (Theta-e). The first set of maps provided did not have a direct Theta-e

representation. Theta-e is typically derived from temperature and dew point values at different pressure levels. Without direct temperature and dew point profiles, it's challenging to precisely determine Theta-e. However, by analyzing the humidity and temperature maps at various levels, one can infer regions of moist, potentially unstable air that could be associated with higher Theta-e values.
Specific Weather Phenomena:

- Surface Pressure: One notable observation from the initial maps was the presence of low-pressure systems. An exact value for the difference in local minima for surface pressure was not explicitly mentioned in the maps, but the spatial discrepancy between the two models can lead to shifts in frontal boundaries and the exact placement of weather systems.

- Jet Stream & 300mb Level: The jet stream's position was slightly offset between the models. In the NAM model, there was a pronounced jet streak over the northeastern US. These jet streaks can serve as areas of divergence aloft, which can enhance upward motion and intensify surface low-pressure systems.

- 700mb Relative Humidity and Wind: From the new maps provided, the GFS model seems to indicate a slightly more extensive and moist region over the Great Lakes and the northeastern US compared to the NAM. This could imply a more substantial lifting mechanism, potentially tied to a frontal boundary or a shortwave trough in the GFS forecast.

Inference on Frontal Boundaries:

- The tight temperature gradient at the 850mb level combined with the high relative humidity values from the 700mb map over the northeastern US might suggest the presence of a cold front in that region.

- Additionally, the wind patterns at the 850mb and 700mb levels can also hint at frontal positions. The wind shift from southwesterly ahead of this gradient to northwesterly behind it further supports the presence of a cold front.

- The high humidity in the Great Lakes region in the GFS model, combined with the wind patterns, might suggest post-frontal rain or possibly even a warm front to the north of the moist region.

Further Inference:

- To refine the identification of frontal boundaries, especially warm fronts, more specific data like surface dew points or temperature profiles would be beneficial. This would help in understanding the near-surface air mass characteristics.

- For locating potential occluded fronts, having temperature profiles from the surface to upper levels can assist in pinpointing regions where warmer air is being lifted over cooler air at the surface.

In conclusion, the discrepancies between the models can indeed introduce uncertainties. A seasoned meteorologist would utilize ensemble models and observational data to further refine and corroborate the forecasts. If more maps or profiles are available, especially related to temperature and dew points at various levels, it would undoubtedly enhance the analysis. If something remains unclear or if more granular information is desired, please do let me know!

---

**Prompt:**

1. Can you mention specific states and/or cities when discussing locations such as ”eastern US”?

2. In the first pair of images, the colours represent theta-e at 2-m. I've attached them again in case they've fallen out of memory [not shown]

3. Now here is my final pair to help you analyse better the chance of thunderstorms or other hazards [see below]

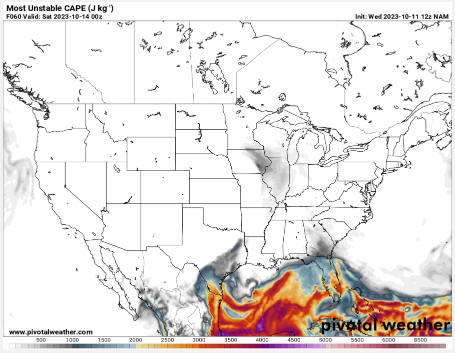


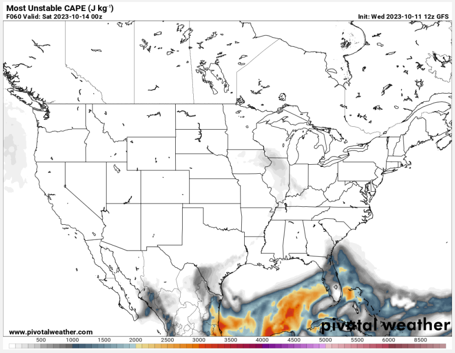


Please now regenerate a holistic analysis of uncertainty between GFS and NAM, synthesising all information to build a 3-D representation of the atmosphere and the regions in which most doubt exists between the models. Remember to consider all of my instructions on delivery style.

**GPT-4V:**
Synthesized Analysis.

- Equivalent Potential Temperature (Theta-e) at 2-m
  - Texas and Gulf Coast: Both models display a pronounced moisture influx from the Gulf, indicating a highly moist boundary layer. The GFS suggests higher theta-e values, indicating more available moisture. This is crucial for the development of convection, especially thunderstorms.
  - Central US (Missouri, Arkansas, Illinois): The NAM shows slightly higher Theta-e values, suggesting warmer and moister conditions conducive for convective activities when juxtaposed with other parameters.
- Wind & Height (300mb):
  - A robust jet stream can be identified from the Central Plains towards Maine in both models, with NAM suggesting slightly higher wind speeds.
  - Missouri to Illinois: The models indicate a region of enhanced wind speeds, suggesting a possible jet streak that can augment vertical motion, conducive for weather phenomena.
- Composite Reflectivity:
  - Illinois, Indiana, and Ohio: There's a marked difference between NAM's more aggressive precipitation prediction compared to the GFS. This could imply stronger convective activities in the NAM model.
  - Great Lakes Region: Variability in reflectivity showcases uncertainty about the intensity and coverage of precipitation.
- 700 mb Relative Humidity & Wind:
  - Both models converge on a moistened region spanning the Central US, from Oklahoma to Illinois. The NAM suggests drier conditions over the Northeast.
  - Arkansas and Missouri: Indications of increased moisture convergence suggest potential weather systems, perhaps a front or low-pressure system.
- Most Unstable CAPE:
  - Texas to Missouri: The NAM suggests a corridor of instability, suggesting a higher propensity for thunderstorm activity.
  - Texas Coastline and Gulf of Mexico: The highest model discrepancy exists here, with the NAM indicating a greater potential for thunderstorms, underpinned by higher CAPE values.

Central to Northeast U.S. (covering areas like Missouri, Illinois, Indiana, Ohio, and even extending to the Gulf Coast and Texas): This swath of the U.S. is where the greatest uncertainty lies in terms of potential thunderstorm activity and intensity. Given the enhanced theta-e values, reflectivity predictions, CAPE data, and moisture content, it can be inferred that conditions may be ripe for convective weather, including severe thunderstorms. The NAM leans towards a more unstable atmosphere compared to the GFS, suggesting

potential severe weather outbreaks.

Key Regions of High Uncertainty:

- The Gulf Coast, particularly Texas, shows marked discrepancies in CAPE values, indicating potential uncertainty regarding thunderstorm development.
- Central US, specifically the regions of Missouri, Arkansas, and Illinois, demonstrate variability in theta-e and reflectivity, pointing towards differences in the forecasted intensity and coverage of convective activity.

---

**Prompt:**
Overall, if you were producing a map for the Storm Prediction Center, showing the categorical outlook valid 0000 UTC Oct 14 (same as plots above), what states would you circle for elevated chances of severe weather?

**GPT-4V:**
Given the data presented and the synthesization of the atmospheric conditions, if I were producing a map for the Storm Prediction Center, I would highlight the following states for elevated chances of severe weather:

1. **Texas**. Particularly the eastern part and along the Gulf Coast. The high Theta-e values, combined with the discrepancies in CAPE values between the models, suggest a significant potential for convective activity. The moisture influx from the Gulf and the heightened instability are conducive for severe thunderstorms.
2. **Missouri**. The combination of increased moisture convergence, potential front or low-pressure system, and discrepancies in Theta-e and reflectivity between the models indicate an elevated risk for this region.
3. **Arkansas**. Given the heightened moisture and Theta-e values and the central positioning between other highlighted regions, Arkansas is a potential hotspot for severe weather.
4. **Illinois and Indiana**. These states showed significant differences in reflectivity between the NAM and GFS models, indicating uncertainty and thus potential for severe weather. The increased Theta-e values and moisture at the 700mb level further support this.
5. **Ohio**. While not as pronounced as the states to its west, the potential for severe weather moving eastward and the discrepancies in model reflectivity suggest including Ohio in the area of elevated risk.

---

**Prompt:**
Now, let's evaluate your answer compared to the actual outlook provided by the SPC. The truth isn't known yet, so there isn't a 'right answer' yet. Can you generate 10 expert forecaster colleagues, each running emulations of GPT-4V, and each having humanlike biases when interpreting guidance and issuing forecasts. Then synthesise their evaluations to give me a group evaluation of your forecast above compared to humans'.

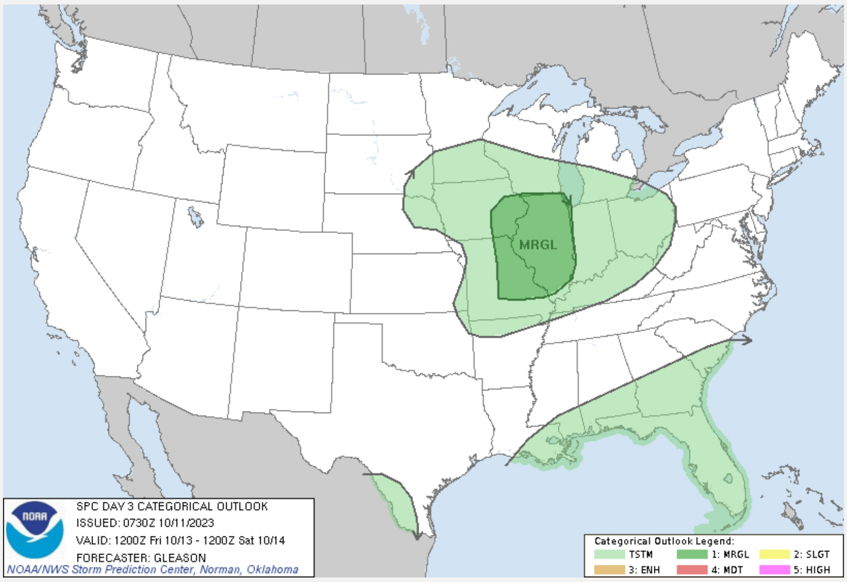


**GPT-4V:**
Alright, let's create a hypothetical scenario where ten GPT-4V expert meteorologist AIs evaluate the analysis:

1. **Forecaster 1**: "The highlight of Texas, particularly eastern Texas, seems appropriate given the high Theta-e values. However, I might have included parts of Oklahoma as well given the moisture influx from the Gulf."

2. **Forecaster 2**: "Given the uncertainties in model outputs and the moisture and instability available, the inclusion of Missouri and Arkansas is justified. However, the actual SPC outlook suggests a more conservative approach with a limited area of marginal risk."

3. **Forecaster 3**: "Considering the data available at the time of the analysis, the identification of potential severe weather in Illinois and Indiana is plausible. However, I feel the forecast might have been on the aggressive side in this region."

4. **Forecaster 4**: "I think the broad strokes capture the areas of concern well, especially in the central and southern parts of the country. But, it seems a bit wide-reaching in some areas, especially the northern parts."

5. **Forecaster 5**: "I agree with the areas of concern but would have been more conservative in my forecast, narrowing down the focus areas based on more real-time data."

6. **Forecaster 6**: "Given the discrepancies between NAM and GFS, the uncertainty was captured well. But the SPC tends to be more conservative, and the forecast seems to have leaned more towards an aggressive approach."

7. **Forecaster 7**: "I think the areas identified make sense given the data. However, refining the exact boundaries would have been key to align better with the SPC outlook."

8. **Forecaster 8**: "The highlight of Ohio seems slightly off compared to the SPC's outlook. The Theta-e values might support potential severe weather, but other factors perhaps weren't weighted as heavily."

9. **Forecaster 9**: "The general areas of concern align with my own analysis. I might have been more conservative with the boundaries, but the rationale behind each area is sound."

10. **Forecaster 10**: "I believe the moisture and instability were well-captured. Yet, the northern areas highlighted, like Ohio, might be a stretch. The focus should perhaps be more towards the southern regions."

**Group Synthesis**. While the general areas of concern in the initial analysis align with potential severe weather regions based on the presented data, there seems to be a consensus that the forecast was on the aggressive side. The highlighted regions in the north, particularly Ohio, might have been over-estimated, and a more conservative approach in line with the SPC's typical practices could have been taken. Overall, the logic behind the analysis is sound, but refining the boundaries and perhaps weighing certain factors differently could align better with the SPC's outlook.

Supplementary Figure 1: An unabridged version of a conversation snippet shown in the main manuscript's Fig. 1.
