# Supplementary material for: Pixels and Predictions: Potential of GPT-4V in Meteorological Imagery Analysis and Forecast Communication
Source: arXiv:2404.15166 source file (2024-09-07)
Supplement: Supplementary file 2 [file z_supp.tex]

\documentclass{article}
\usepackage{pdfpages}

\begin{document}

% Include the PDF
\begin{center}
    \Large SUPPLEMENTARY MATERIAL
\end{center}
\includepdf[pages=-]{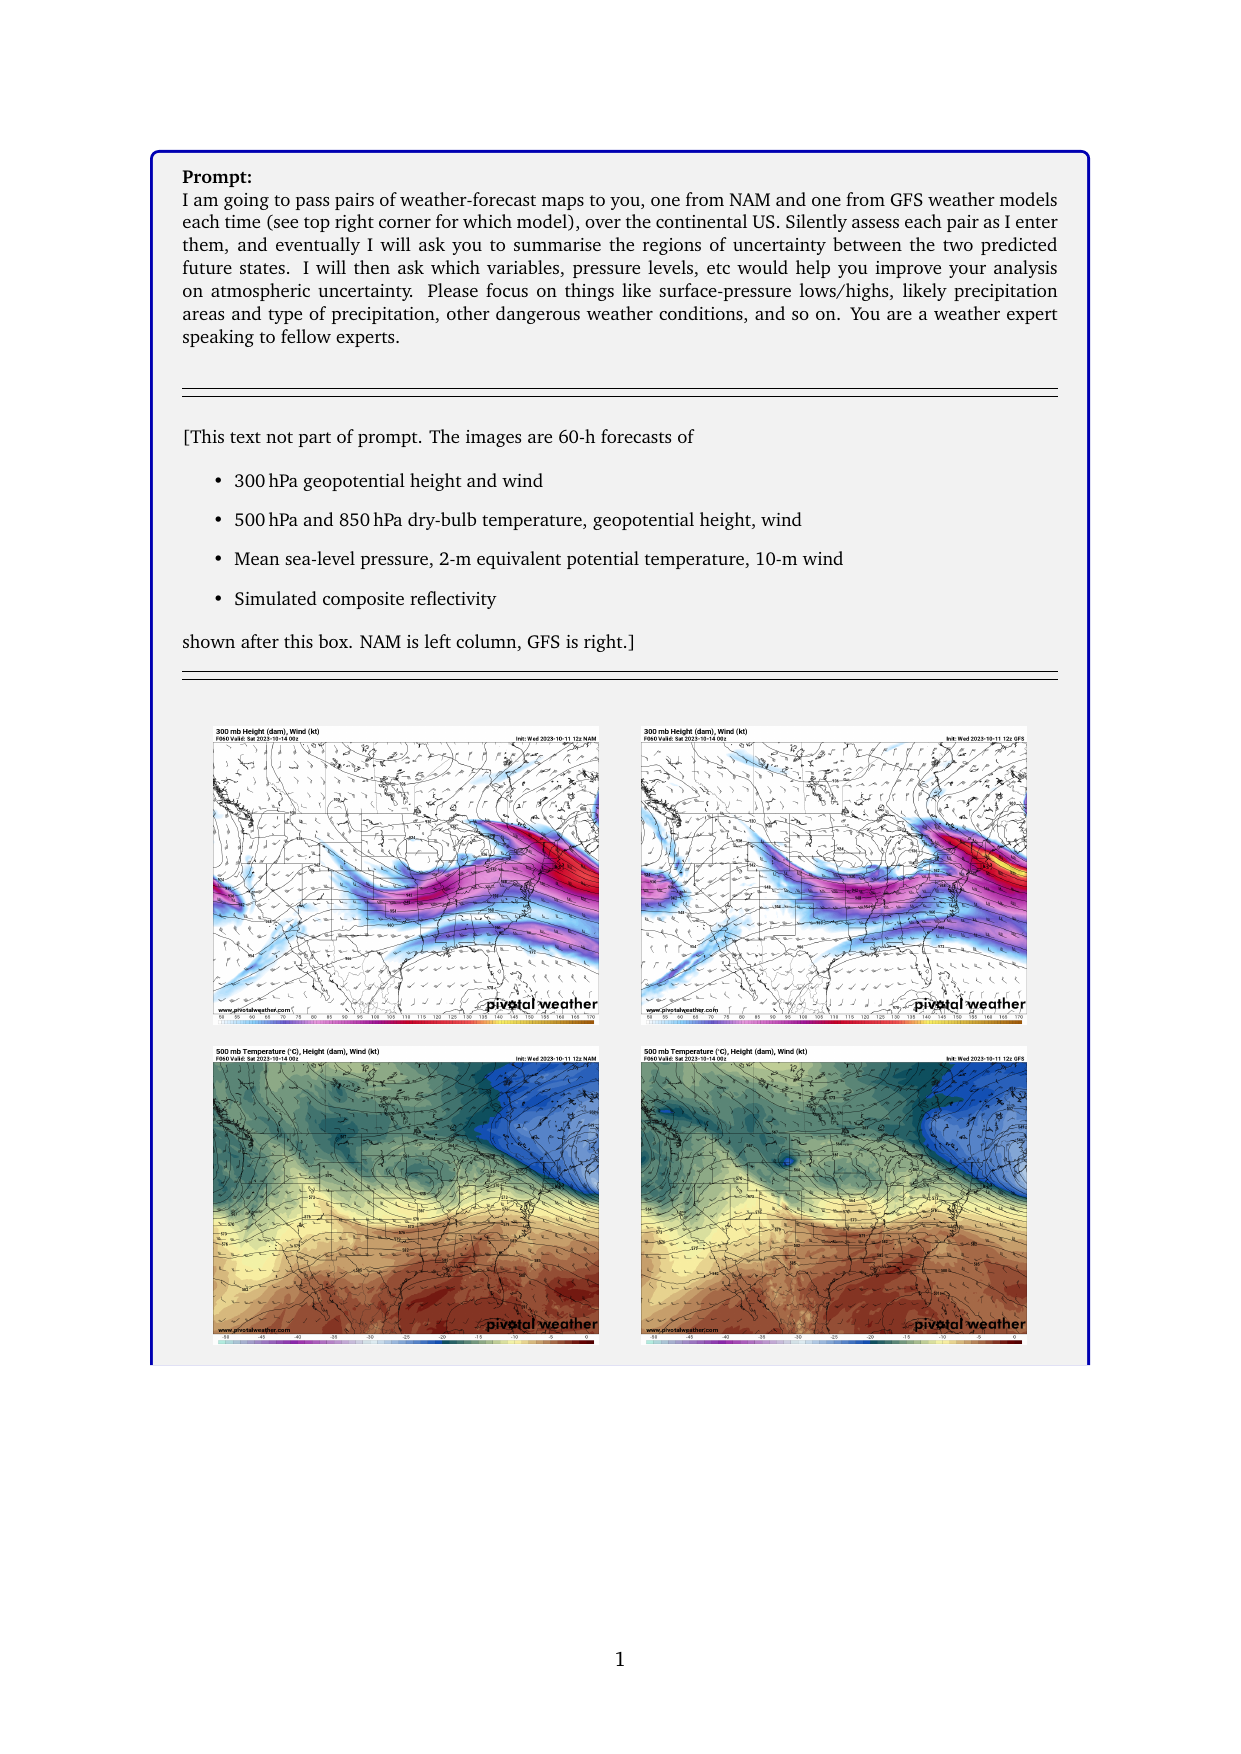}

\end{document}
